# Supplementary material for: ProcVLM: Learning Procedure-Grounded Progress Rewards for Robotic Manipulation
Source: arXiv:2605.08774 source file (2026-09-26)
Supplement: Supplementary file 1 [file neurips_others.tex]

\clearpage
\section{Broader Impacts, Compute Resources, Existing Assets and Licenses}

\textbf{Broader impacts.} ProcVLM is intended as a research-stage model for procedure-aware reward modeling in robotic manipulation. It may reduce the need for manually designed rewards and provide interpretable dense feedback for manipulation tasks, supporting failure diagnosis and reward-guided policy optimization. However, inaccurate progress estimates may misguide downstream policy learning, especially if the reward signal is used directly in physical robotic systems without downstream adaptation to the target environment and additional safety checks. The current work focuses on benchmark evaluation and research-stage optimization rather than safety-critical deployment. Any real-world use of ProcVLM-derived rewards should require task-specific validation, explicit safety checks, and human oversight.

\begin{table}[h]
\centering
\caption{Compute resources used in the main experiments.}
\label{tab:compute_resources}
\footnotesize
\setlength{\tabcolsep}{3pt}

\begin{tabularx}{\linewidth}{@{}L{0.15\linewidth} L{0.17\linewidth} L{0.17\linewidth} L{0.07\linewidth} Y@{}}
\toprule
Experiment & Run & Hardware & Time & Notes \\
\midrule

Annotation synthesis
& Full annotation pipeline
& 8$\times$ H100 80GB
& 20d
& Batched VLM inference with vLLM and LMDeploy. \\

\midrule
\multirow{2}{0.15\linewidth}{\RaggedRight ProcVLM training}
& Stage 1 pretraining
& 16$\times$ H100 80GB
& 5d
& DeepSpeed ZeRO-2. \\
& Stage 2 refinement
& 16$\times$ H100 80GB
& 3d
& DeepSpeed ZeRO-2 with offload. \\

\midrule
\multirow{2}{0.15\linewidth}{\RaggedRight ProcVQA evaluation}
& Qwen3.5-27B
& 8$\times$ H100 80GB
& 40h
& vLLM inference on ID/OOD splits. \\
& Qwen3-235B-A22B
& 8$\times$ H100 80GB
& 30h
& vLLM inference on ID/OOD splits. \\

\midrule
Reward-model evaluation
& Robometer / RoboDopamine
& 4$\times$ A6000 40GB
& 5h
& Total evaluation time on the ProcVQA progress-estimation subset across both splits. \\

\midrule
RoboFAC adaptation
& One-shot adaptation
& 4$\times$ A6000 40GB
& 2h
& Single-setting adaptation for Robometer and ProcVLM. \\

\midrule
\multirow{2}{0.15\linewidth}{\RaggedRight Reward-guided optimization}
& LIBERO RFT
& 4$\times$ A6000 40GB
& 8h
& Policy fine-tuning experiments in simulation. \\
& Real-robot RFT
& 4$\times$ A800 80GB
& 26h
& Policy fine-tuning experiments on real-robot data. \\

\bottomrule
\end{tabularx}
\end{table}

% \begin{table}[H]
% \centering
% \caption{Summary of existing assets used in this work. We cite the original sources and follow their official licenses or terms of use.}
% \label{tab:existing_assets}
% \footnotesize
% \setlength{\tabcolsep}{3pt}
% \renewcommand{\arraystretch}{1.12}
% \begin{tabularx}{\linewidth}{@{}L{0.18\linewidth} L{0.34\linewidth} L{0.25\linewidth} Y@{}}
% \toprule
% Category & Assets & Usage & License / Terms \\
% \midrule

% Pretrained models
% & Qwen3-VL, Qwen3.5, InternVL3.5
% & Backbone, annotation, and evaluation
% & Official model licenses and terms. \\

% Embodied datasets
% & DROID, BridgeData V2, Fractal, and other datasets listed in Appendix~B
% & ProcCorpus construction
% & Original dataset licenses and terms; raw data are not redistributed. \\

% Benchmarks
% & LIBERO, RoboFAC
% & Simulation evaluation and one-shot reward-model adaptation
% & Original benchmark licenses and terms. \\

% Reward-model baselines
% & Robometer, RoboDopamine
% & Reward-model comparisons
% & Original model/code licenses and terms. \\

% Software
% & vLLM, LMDeploy, DeepSpeed, Transformers
% & Inference, annotation, distributed training, and model implementation
% & Official open-source licenses. \\

% \bottomrule
% \end{tabularx}
% \end{table}

\begin{table}[H]
\centering
\caption{Summary of existing assets used in this work. We cite the original sources and follow their official licenses or terms of use. Raw third-party data are not redistributed.}
\label{tab:existing_assets}
\footnotesize
\setlength{\tabcolsep}{3pt}

\begin{tabularx}{\linewidth}{@{}L{0.12\linewidth} L{0.21\linewidth} L{0.21\linewidth} Y@{}}
\toprule
Category & Assets & Usage & License / Terms \\
\midrule

Pretrained models
& Qwen3-VL, Qwen3.5, InternVL3.5
& Backbone, annotation, and evaluation
& Apache-2.0 for Qwen3-VL and Qwen3.5 checkpoints; Apache-2.0 for InternVL3.5 checkpoints, with InternVL code under MIT. \\
\midrule

Embodied datasets
& DROID, BridgeData V2
& ProcCorpus construction
& CC BY 4.0; used according to the original dataset terms, with no raw-data redistribution. \\
\midrule

Embodied datasets
& Fractal / RT-1 and selected Open X-Embodiment subsets
& ProcCorpus construction
& Open X-Embodiment materials under CC BY 4.0 and software under Apache-2.0; individual contributed datasets are cited following upstream metadata. \\
\midrule

Embodied datasets
& RH20T and Table30
& ProcCorpus construction
& RH20T uses mixed terms: RH20T-C under CC BY-SA 4.0 and RH20T-NC under CC BY-NC 4.0. Table30 is used under its source hosting terms; its public dataset card does not specify an explicit license at the time of writing. \\
\midrule

Benchmarks
& LIBERO, RoboFAC
& Simulation evaluation and one-shot reward-model adaptation
& LIBERO code under MIT; RoboFAC dataset under MIT. \\
\midrule

Reward-model baselines
& Robometer, RoboDopamine
& Reward-model comparisons
& Robometer code/model release under MIT; RoboDopamine code under Apache-2.0. \\
\midrule

Software
& vLLM, LMDeploy, DeepSpeed, Transformers, Evo-RL
& Inference, annotation, distributed training, and model implementation
& Apache-2.0. \\

\bottomrule
\end{tabularx}
\end{table}
